# Supplementary material for: Calculating the Single-Particle Many-body Green's Functions via the Quantum Singular Value Transform Algorithm
Source: arXiv:2307.13583 source file (2023-07-25)
Supplement: Supplementary file 1 [file DMFT_appendix.tex]

% \section{Dynamical Mean Field Theory} \label{sec:DMFT}
% % https://d-nb.info/998896241/34
% % https://physics.stackexchange.com/questions/680370/dynamical-mean-field-theory-dmft-does-not-take-into-account-spacial-correlatio
% For many strongly correlated systems it is possible to write down an effective Hamiltonian describing the system. However, due to strong correlations are difficult to solve. Dynamical mean field theory (DMFT), captures the physics of a many body problem via a single impurity that is coupled self-consistently to a Fermonic host (bath). The underlying principle is as the number of sites in a problem goes to infinity, the central limit theorem means fluctations from site-to-site can be neglected. Instead the influence of a site from all others can be replaced by an effective medium -  i.e. the degrees of freedom on the other sites will be integrated out as an external bath interacting with the chosen site. Overall, the many-body problem has been transformed into a quantum impurity problem i.e. a single impurity site interacting with a bath. The crux of DMFT is that the self-energy of a system becomes $k$-independent in the limit of infinite dimensions. This means that the self-energy, that is the correction to the noninteracting Green's function, is local. If the self-energy can be determined and the noninteracting Green's function is known then the full interacting Green's function can be determined - where local fluctuations are treated exactly and the problem is solved.

% In the context of the Hubbard model, in the limit of infinite coordination number (nearest neighbours) DMFT will model the system exactly. DMFT achieves this by decoupling strongly correlated lattice sites into sites interacting with a mutual bath, where the bath parameters are determined self-consistently. 

% % The self-energy of the impurity is first determined and the full Green's function determined and compared to a previous iteration. If the full Green's function remains unchanged (converged) then the algorithm is finished, otherwise the bath parameters are updated and the process is repeated.

% % Crucially, DMFT is derived in the limit of infinite lattice coordination; however, for finite dimensions it can still provide good approximations and allow interesting phenomena to be explored. REFS needed
