# Supplementary material for: Calculating the Single-Particle Many-body Green's Functions via the Quantum Singular Value Transform Algorithm
Source: arXiv:2307.13583 source file (2023-07-25)
Supplement: Supplementary file 2 [file app_block_encoding_circuits.tex]

% \section{Block Encoding Circuits} \label{sec:LCU_circuits}

% In this appendix we show how to construct the quantum circuits to block encoded any complex operator $A$ (equation \ref{eq:LCU_A} in the main text) via the linear combination of unitaries technique. For ease of reading, we repeat the definition of $A$ here:

% \begin{equation}
% \begin{aligned}
% 	A &= \sum_{i=0}^{d-1} \alpha_{i} U_{i}, \: \: \| A\| \leq \sum_{i=0}^{d-1} \bigg( |\alpha_{i}| \cdot \underbrace{\| U_{i}\|}_{=1} \bigg) = \sum_{i=0}^{d-1} |\alpha_{i}| = \|A \|_{1},
% 	\end{aligned}
% \end{equation}
% where, without loss of generality, all $\alpha_{i}>0$ and $\alpha_{i} \in \mathbb{R}$ by absorbing any complex phases and signs into the unitaries  $U_{j}$ \cite{childs2012hamiltonian, low2017optimal, ralli2021implementation}.  Given a list of $\alpha_{i}$ and each $U_{i}$, which are assumed to be easy to implement as controlled operations on a quantum device, the block encoding can be constructed using the oracles \cite{ low2017optimal, ralli2021implementation}:

% \begin{equation}
%  \label{eqn:prep_oracle}
% \begin{aligned}
% 	PREP &= \sum_{i=0}^{d-1} \sqrt{\frac{\alpha_{i}}{ \| A\|_{1}}} \ket{i}\bra{0}_{p}+ \hdots = \begin{bmatrix}
% \big(\frac{\alpha_{0}}{\|A\|_{1}}\big)^{1/2} & \cdot & \hdots \\ 
% \big(\frac{\alpha_{1}}{\|A\|_{1}}\big)^{1/2} & \cdot & \hdots  \\ 
% \vdots &  \ddots & \hdots   \\ 
% \big(\frac{\alpha_{d-1}}{\|A\|_{1}}\big)^{1/2} & \cdot  &  \hdots
% \end{bmatrix}
% 	\end{aligned}
% \end{equation}
% and
% \begin{equation}
%  \label{eqn:select_oracle}
% \begin{aligned}
% 	U_{\text{select}} &= \sum_{i=0}^{d-1} \Big( \ket{i}\bra{i}_{p} \otimes U_{i} \Big).
% 	\end{aligned}
% \end{equation}
% Here subscript $s$ denotes the system register and $p$ the prep (ancilla) register.  The number of prep qubits required will be $n_{p}=\lceil \log_{2}(d)\rceil$.

% The $PREP$ or ``Prepare'' oracle  is a unitary that prepares the state  $\ket{P} = \sum_{i=0}^{d-1} \sqrt{\frac{\alpha_{i}}{\|A\|_{1}} }\ket{i}$ from the all zero state on the ancilla register - i.e. $\ket{\bar{0}} \mapsto \ket{P}_{prep}$.  This is why in equation \ref{eqn:prep_oracle} only the first column is defined. As dicussed in \cite{ralli2021implementation}, the other columns can be anything so long $P$ remains unitary.  This means there is a lot of choice in how to construct this operator. If one simply finds the quantum circuit to do $\ket{\bar{0}}_{a} \mapsto \ket{P}_{a}$,  then the circuits action on the other basis states are automatically accounted for and the whole of $PREP$ will be defined \cite{ralli2021implementation}. The only quantum circuit requirement is being able to generate any real quantum state from the all zero state on the prep register.There are many different proposals on how to prepare arbitrary quantum states \cite{Long2001, Mottonen2005, Markov2006prep, Araujo2021}. Following the approaches given in both \cite{Markov2006prep, Araujo2021}, a real quantum state can be generated using multiplexed $R_{y}$ rotations with the number of single qubit and CNOT gates scaling as $\mathcal{O}(2^{n_{prep}})$ respectively. As the number of $prep$ qubits scales logarithmically with the number of terms in $A$: $\mathcal{O}(log_{2}|A|)$. The number of single qubit and CNOT gates will scale as $\mathcal{O}(|A|)$ for the $PREP$ part of the block encoding circuit. 

% The desired LCU block encoding is achieved by performing $PREP^{\dagger} U_{select}PREP$ and post selecting on the all zero state on the prep qubit register. We can check this via the following proof \cite{ low2017optimal}:

% \input{sections/block_circuit_picture} 

% \begin{equation}
% \begin{aligned}
% \bigg[ \bra{0}_{p} \otimes I_{s} \bigg] (PREP^{\dagger} \otimes I_{s} ) U_{\text{select}} \big(   PREP \otimes I_{s}\big)\bigg[ \ket{0}_{p} \otimes I_{s} \bigg] &=\bigg[ \bra{P}_{p} \otimes I_{s} \bigg] U_{\text{select}} \bigg[ \ket{P}_{p} \otimes I_{s} \bigg] \\
% &=  \bigg[ \bra{P}_{p} \otimes I_{s} \bigg] \Bigg( \sum_{i=0}^{d-1} \sqrt{\frac{\alpha_{i}}{\|A\|_{1}} }\ket{i}\otimes U_{i}  \Bigg) \\
%  &=  \bigg[ \bra{P}_{p} \otimes I_{s} \bigg] \Bigg( \sum_{i=0}^{d-1} \sqrt{\frac{\alpha_{i}}{\|A\|_{1}} }\ket{i}\otimes U_{i}  \Bigg) \\
% 	&= \Bigg( \sum_{k=0}^{d-1} \sqrt{\frac{\alpha_{k}}{\|A\|_{1}} }\bra{k}\otimes I_{s}  \Bigg) \Bigg( \sum_{i=0}^{d-1} \sqrt{\frac{\alpha_{i}}{\|A\|_{1}} }\ket{i} \otimes U_{i}  \Bigg) \\
% 	&= \sum_{i=0}^{d-1}\sum_{k=0}^{d-1} \frac{\sqrt{\alpha_{i}\alpha_{k}}}{\|A\|_{1}} \bra{k} i \rangle \otimes U_{i} \\
% 	&= \frac{1}{\|A\|_{1}} \sum_{i=0}^{d-1} \alpha_{i} U_{i}
% 	\end{aligned}
% \end{equation}
% and is implemented according to the circuit in Figure \ref{fig:block_encode_circ}.

% In this work, the LCU is given as a linear combination of Pauli operators. The ``SELECT'' operator ($U_{select}$) applies a controlled version of each of these Pauli operators on the system register, controlled by the prep register. This requires performing multi-control Pauli operators with phases $\{ i,-i,1,-1 \}$. Following the work in \cite{ralli2021implementation}, this can achieved using the template given in Figure \ref{fig:cntrl_P_gate}. The relevant phases are then obtained via the following identities:

% \begin{subequations}
%  \label{eq:pauli_phases}
%     \begin{equation}
%     \label{eq:neg_sign}
% 	-Z =XZX,
%     \end{equation}
%     %%
% \begin{equation}
%     \label{eq:imag}
% R_{z}(\mp \pi)= e^{\mp i \frac{\pi}{2}Z}  = \pm i Z.
% \end{equation}
% \end{subequations}
% which can be implemented in circuit according to Figure \ref{fig:phaseZgates}. By performing a change of basis on certain qubits, using the gates $\{S, S^{\dagger}, H \}$, the circuit proposed in Figure \ref{fig:cntrl_P_gate} can be used to generate any multicontrol Pauli operator with a $\pm 1, \pm i$ phase.

% To determine the overall circuit cost to implement  $U_{select}$ (equation \ref{eqn:select_oracle} and Figure \ref{fig:block_encode_circ}), we need to determine the cost of implementing a multicontrol $Z$ gate and multicontrol $R_{z}$ gate. Following the approach proposed by Silva and Park, any $n$-control single qubit gate can be decomposed with $\mathcal{O}(n^{2})$ single qubit and CNOT gates with linear depth \cite{da2022linear}. If this construction is decomposed into $CNOT$ and $U3$ gates, then $4 n^{2} - 4 n + 2$  $CNOT$ and $4 n^{2} - 2$ $U3$ gates are required. For $n$-control single qubit $Z$ gates with $n \leq 6$, the approach outlined in \cite{bullock2003smaller} requires fewer two-qubit gates, where the number of single qubit and CNOT gates required is $2^{n+1}-1$ and $2^{n+1}-2$ respectively. In general, using the approaches discussed here the cirucit cost to perform a multicontrol Pauli operator via the template in Figure  \ref{fig:cntrl_P_gate} will scale as $O(2n_{s})$ change of basis gates, $O(2[n_{s}-1])$ CNOT gates and $O(n_{c}^{2})$ CNOT and single qubit gates for the multicontrol $i^{k}Z$ gate. Here $n_{c}$ is the number of control qubits and $n_{s}$ is the number of `system' qubits the Pauli operator acts on. The cost per $n_{c}$-controlled Pauli operator is  quadratic in single and two qubit gates. The overall cost of implementing $U_{select}$ vi this approach depends on the number of $n_{c}$-controlled Pauli operator that are performed. Looking at equation  \ref{eqn:select_oracle}, the number of single and CNOT gates will scale as $O(d[n_{c}^{2}+n_{s}])$ single and two qubit gate. As $d = |A|$ and $n_{c} = \lceil \log_{2}(|A|) \rceil$, we can write the final cost as  $O\big( |A| \lceil \log_{2}(|A|) \rceil^{2}+ |A|n_{s} \big)$.


% \begin{figure}[t]
% \centering
% \input{circuits/phase_ZZZ_gate.tikz}
% \caption{Circuit template to perform $n$-control Pauli operator composed of Pauli $Z$ and $I$ single qubit matrices. Figure \ref{fig:imagZgate} provides the circuit construction for the multicontrol $i^{k}Z$ gate.}
% \label{fig:cntrl_P_gate}
% \end{figure}

% \begin{figure}
%      \centering
%      \begin{subfigure}[b]{0.9\textwidth}
%          \centering
%          \input{circuits/negZ_gate.tikz}
%          \caption{$k=2$}
%          \label{fig:negZgate}
%      \end{subfigure}
%      \hfill
%      \begin{subfigure}[b]{0.9\textwidth}
%          \centering
%          \input{circuits/iZ_gate.tikz}
%          \caption{$k \in \{1,3\}$}
%          \label{fig:imagZgate}
%      \end{subfigure}

%     \caption{Circuit construction of multicontrol single qubit $i^{k}Z$ gate, for $k \in \{0,1,2,3\}$. Circuit for $k=0$ is not shown , as it is the trivial case of a multicontrol single qubit $Z$ gate. This is the same as Figure \ref{fig:negZgate} with both $X$ gates removed.}
%     \label{fig:phaseZgates}
% \end{figure}
